# Supplementary material for: Resonance: Learning to Predict Social-Aware Pedestrian Trajectories as Co-Vibrations
Source: arXiv:2412.02447 source file (2025-03-10)
Supplement: Supplementary file 2 [file s1_displayissues.tex]

%%%%%%%%%%%%%%%%%%%%%%%
%% Author: Conghao Wong
%% Date: 2024-11-18 16:04:10
%% LastEditors: Conghao Wong
%% LastEditTime: 2024-11-19 15:31:25
%% Github: https://cocoon2wong.github.io
%% Copyright 2024 Conghao Wong, All Rights Reserved.
%%%%%%%%%%%%%%%%%%%%%%%

\documentclass[../../paper.tex]{subfiles}

\begin{document}

\twocolumn[{%
    \renewcommand\twocolumn[1][]{#1}%
    \maketitlesupplementary
    \appendix
    \section{Special Notes: Image Display Issues}
    \begin{center}
        \centering
        \includegraphics[width=1.0\linewidth]{../../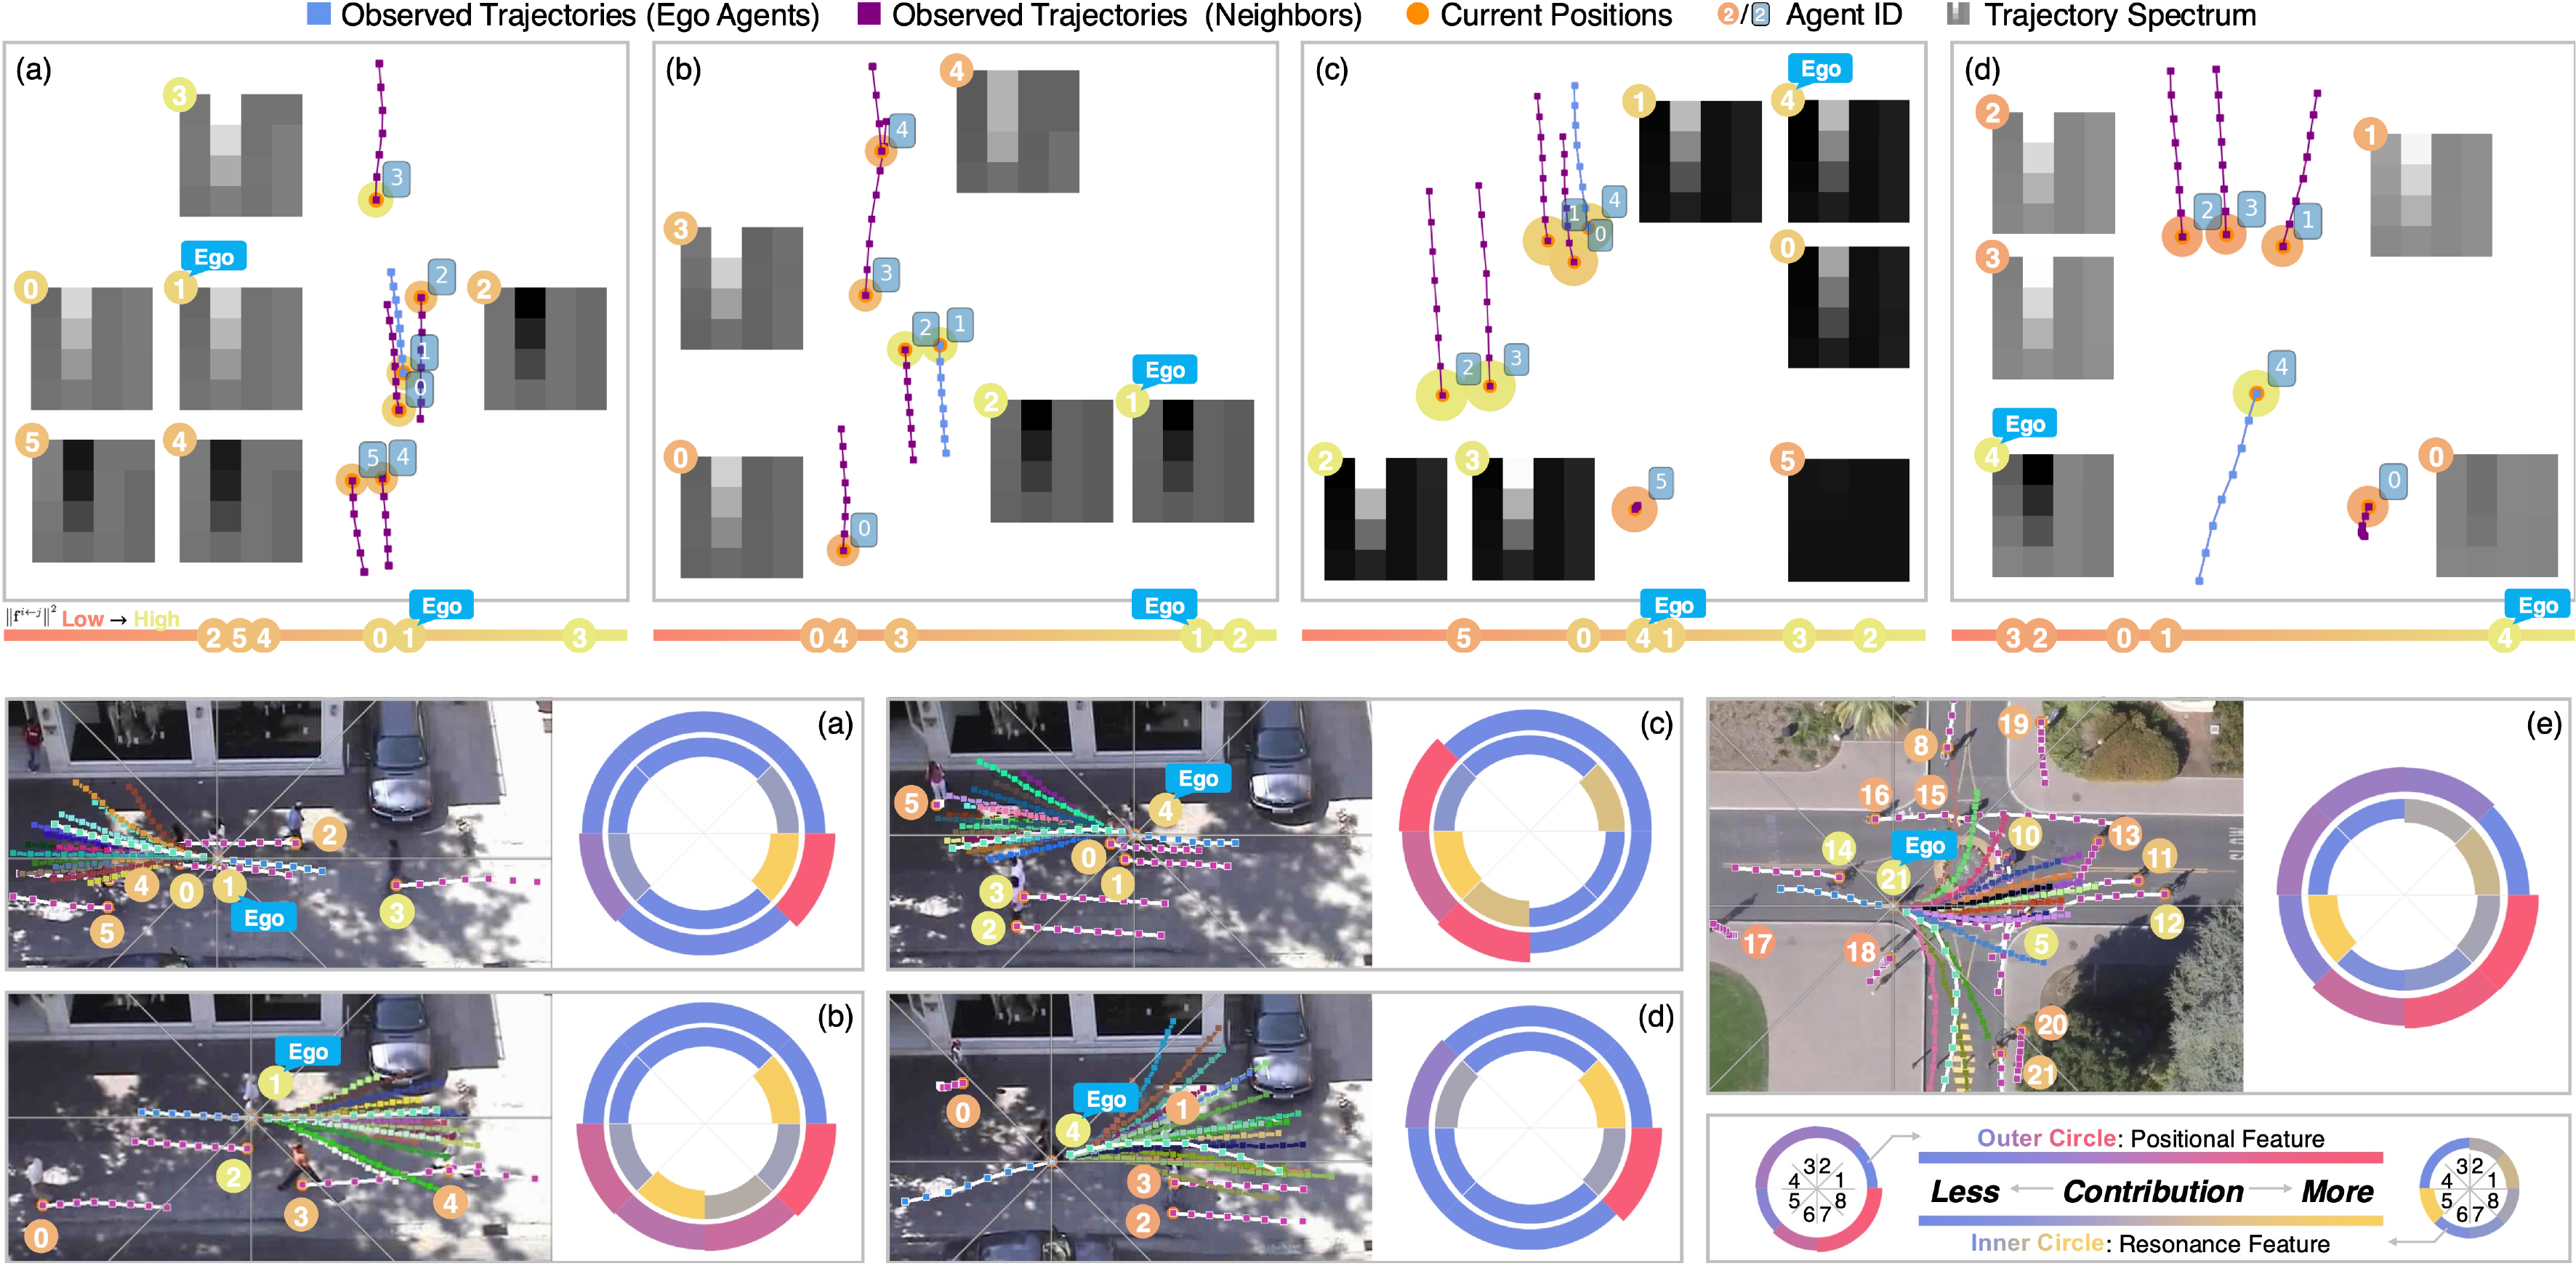}
        \captionof{figure}{
            PNG versions of the images that may not correctly displayed in the main file, corresponding to the original Figs. 8 and 9.
        }
        \label{fig_pngimages}
    \end{center}%
}]

\begin{figure}[h]
    \centering
    \includegraphics[width=1.0\linewidth]{../../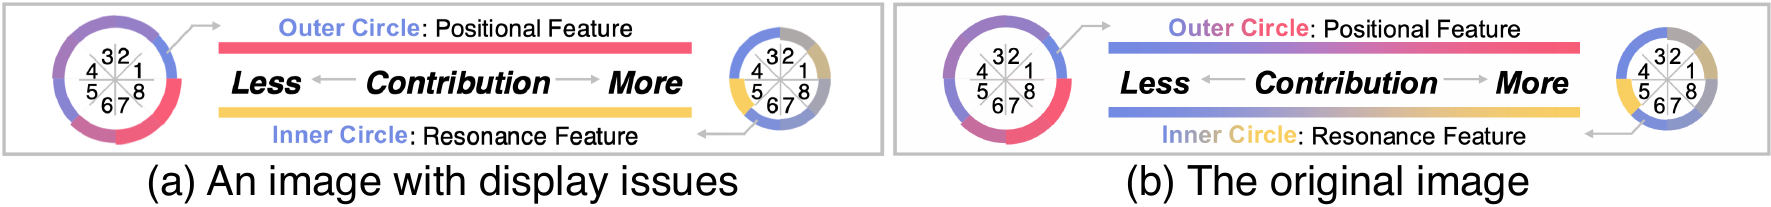}
    \caption{
        Illustration of image display issues in the main document.
        Some images (especially those with color gradients) may not correctly displayed in some unknown situations, shown in subfigure (a), leading to potential misunderstandings.
    }
    \label{fig_imageissue}
\end{figure}

\begin{figure}[h]
    \centering
    \includegraphics[width=1.0\linewidth]{../../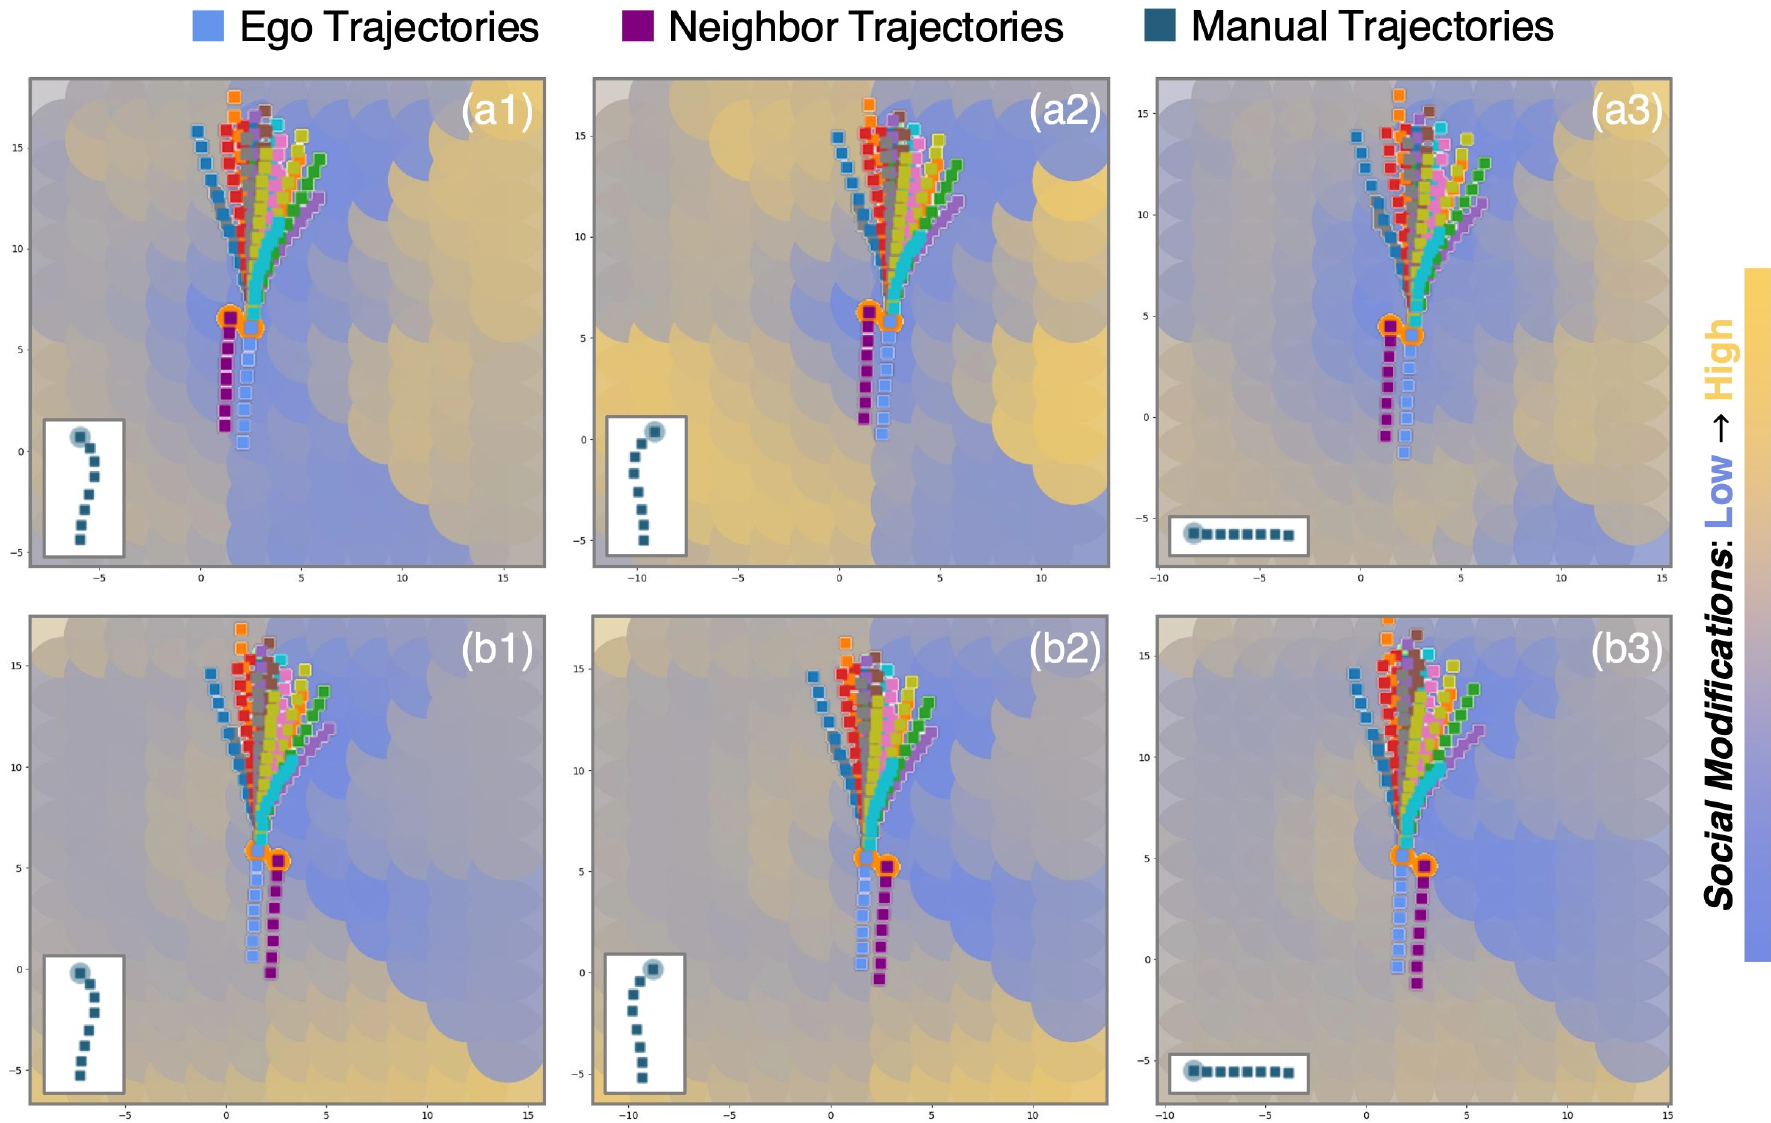}
    \caption{
        PNG version of the image that may not correctly displayed in the main file, corresponding to the original Fig. 10.
    }
    \label{fig_pngimages2}
\end{figure}

As illustrated in \FIG{fig_imageissue}, after submitting the main file, we found that some images inside may have display problems in some unknown situations, especially those involving transparency and color gradients.
We use PowerPoint for Mac (version 16.91 (24111020)) to draw all the images (and export them as PDF files to build paper with PDFLatex).
In Google Chrome (or a PDF reader with the same kernel), these images display fine in the main PDF file.
However, after our testing, when opened in the macOS preview app or Safari, these images may display incorrectly and do not show all the gradient bars (which mostly are used to indicate the value of some metrics).
Therefore, to minimize misunderstandings, we have attached some images that have been significantly impacted here, including the original Figs. 8 and 9 in \FIG{fig_pngimages}, and the original Fig. 10 in \FIG{fig_pngimages2}.
We also put all these images in the supplementary folder.
Please note that \textbf{\emph{no changes have been made to these images}}, and we only convert them to PNG files here (they should look the same as what displayed in Google Chrome).

\end{document}
