# Supplementary material for: Resonance: Learning to Predict Social-Aware Pedestrian Trajectories as Co-Vibrations
Source: arXiv:2412.02447 source file (2025-03-10)
Supplement: Supplementary file 3 [file s1_fig_imageissue.tex]

%%%%%%%%%%%%%%%%%%%%%%%
%% Author: Conghao Wong
%% Date: 2024-10-23 16:03:42
%% LastEditors: Conghao Wong
%% LastEditTime: 2024-11-18 15:18:01
%% Github: https://cocoon2wong.github.io
%% Copyright 2024 Conghao Wong, All Rights Reserved.
%%%%%%%%%%%%%%%%%%%%%%%

\documentclass[../../paper.tex]{subfiles}

\begin{document}

\begin{figure}[h]
    \centering
    \includegraphics[width=1.0\linewidth]{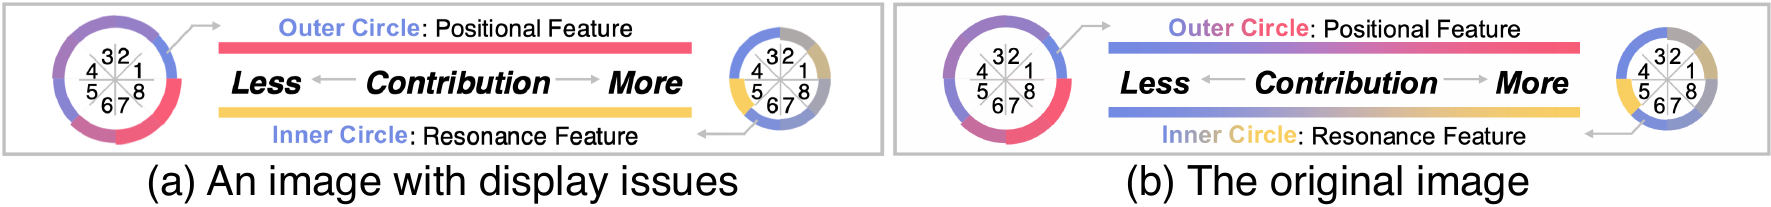}
    \caption{
        Illustration of image display issues in the main document.
        Some images (especially those with color gradients) may not correctly displayed in some unknown situations, shown in subfigure (a), leading to potential misunderstandings.
    }
    \label{fig_imageissue}
\end{figure}

\end{document}
