# Supplementary material for: Resonance: Learning to Predict Social-Aware Pedestrian Trajectories as Co-Vibrations
Source: arXiv:2412.02447 source file (2025-03-10)
Supplement: Supplementary file 4 [file s1_fig_pngimages2.tex]

%%%%%%%%%%%%%%%%%%%%%%%
%% Author: Conghao Wong
%% Date: 2024-11-18 14:44:57
%% LastEditors: Conghao Wong
%% LastEditTime: 2024-11-18 18:26:00
%% Github: https://cocoon2wong.github.io
%% Copyright 2024 Conghao Wong, All Rights Reserved.
%%%%%%%%%%%%%%%%%%%%%%%

\documentclass[../../paper.tex]{subfiles}

\begin{document}

\begin{figure}[h]
    \centering
    \includegraphics[width=1.0\linewidth]{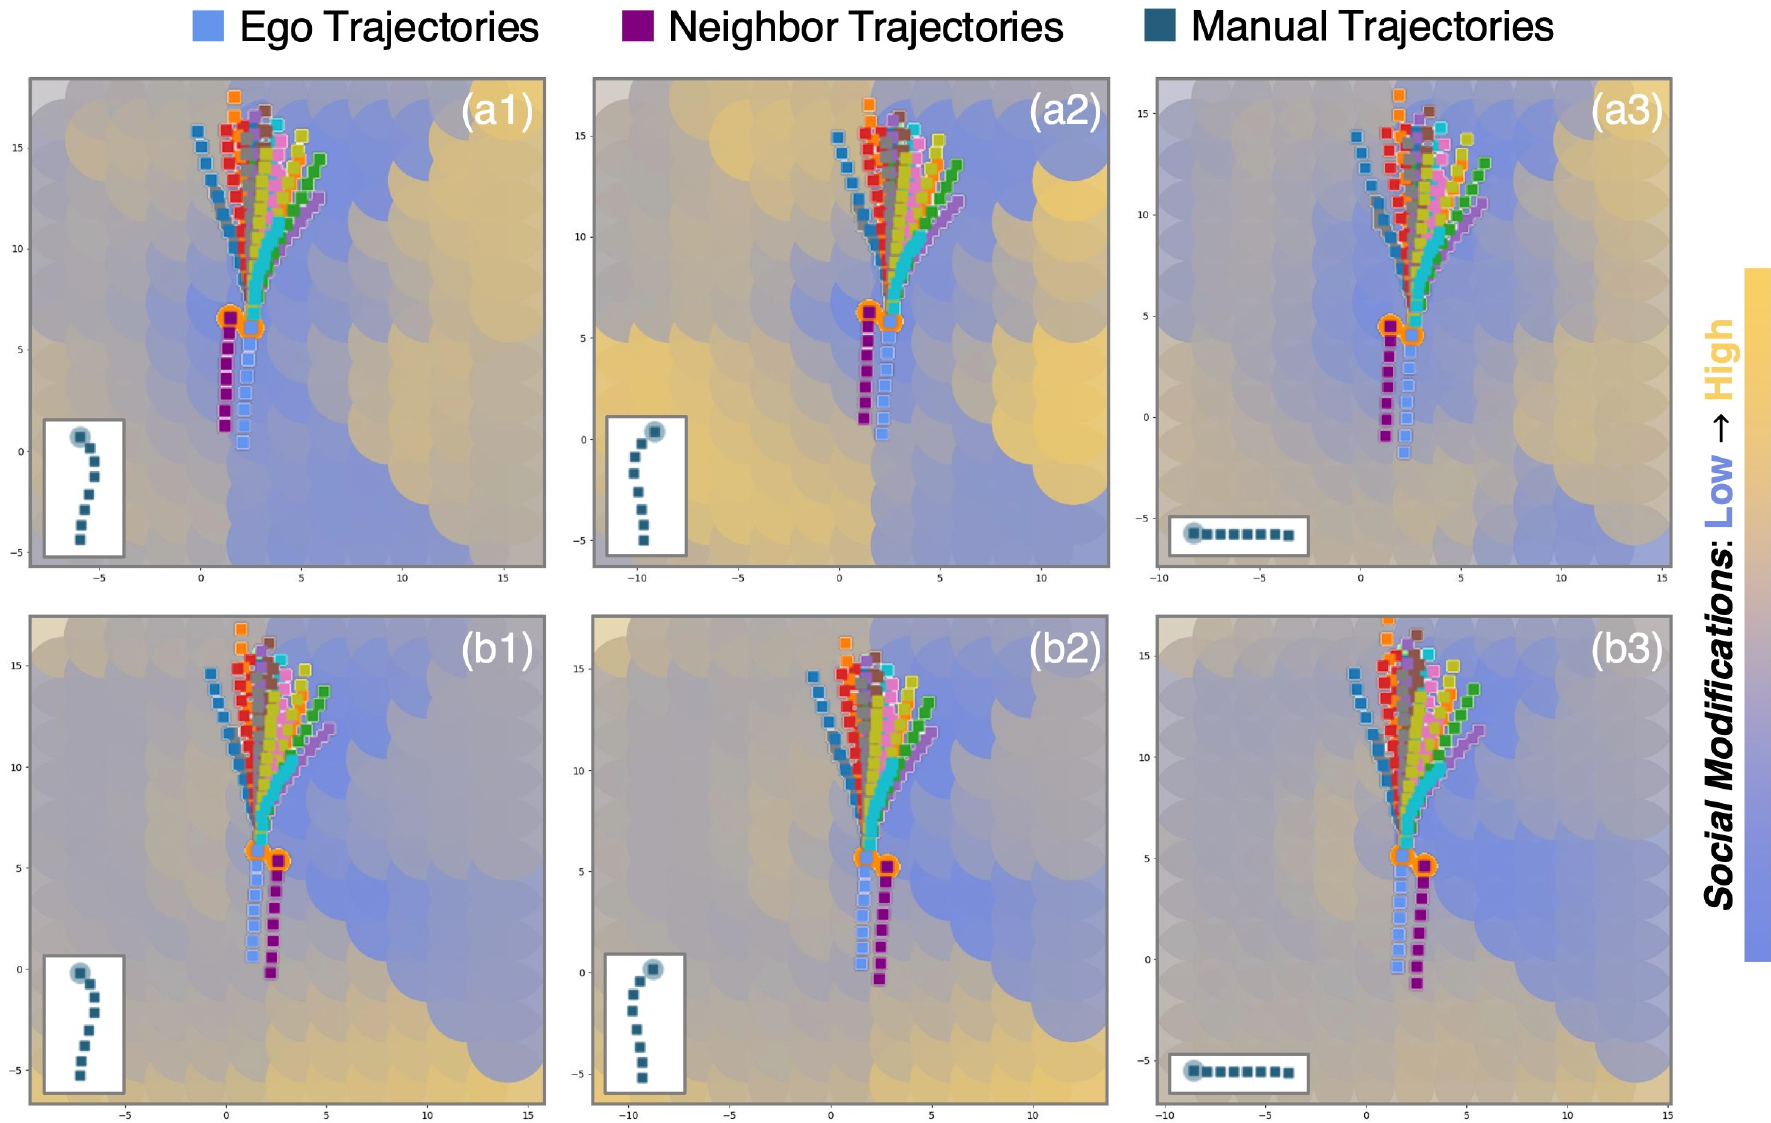}
    \caption{
        PNG version of the image that may not correctly displayed in the main file, corresponding to the original Fig. 10.
    }
    \label{fig_pngimages2}
\end{figure}

\end{document}
