# Supplementary material for: Resonance: Learning to Predict Social-Aware Pedestrian Trajectories as Co-Vibrations
Source: arXiv:2412.02447 source file (2025-03-10)
Supplement: Supplementary file 7 [file s3t1_efficiency.tex]

%%%%%%%%%%%%%%%%%%%%%%%
%% Author: Conghao Wong
%% Date: 2024-10-16 09:16:58
%% LastEditors: Conghao Wong
%% LastEditTime: 2024-11-22 10:20:02
%% Github: https://cocoon2wong.github.io
%% Copyright 2024 Conghao Wong, All Rights Reserved.
%%%%%%%%%%%%%%%%%%%%%%%

\documentclass[../../paper.tex]{subfiles}

\begin{document}

\begin{table}[tbp]
    \centering
    \footnotesize
    \begin{tabular}{lccccc}
        \toprule
        Method & Performance (SDD) & $t_{\mathrm{1}}$ & $t_{\mathrm{1k}}$ & Parameter \\

        \midrule
        \EVMODEL~\EVCITE & 6.57/10.49 & \C{28} & \C{112} & \C{1,976,864} \\
        \SCMODEL~\SCCITE & 6.54/10.36 & \C{34} & \C{119} & \C{1,989,536} \\
        \SCPMODEL~\SCPCITE & 6.44/10.22 &  41 & 126 & 1,990,177 \\

        \MODELSHORT~(variation a2) & 6.93/10.26 & \C{29} & \C{91} & 2,046,428 \\
        \MODELSHORT~(variation a8) & 6.33/10.45 & \C{34} & 211 & \C{1,242,924} \\
        \MODELSHORT~(full) & 6.27/10.02 & 56 & 263 & 3,149,192 \\

        \bottomrule
    \end{tabular}
    \caption{
        Comparisons of the average inference times (on an Apple M1 Mac mini (2020, 8GB Memory)) under the batch size of 1 and 1000 (denoted as $t_{\mathrm{1}}$ and $t_{\mathrm{1k}}$ correspondingly, reported in milliseconds), and parameter amount.
    }
    \label{tab_efficiency}
  \end{table}

\end{document}
