# Supplementary material for: Resonance: Learning to Predict Social-Aware Pedestrian Trajectories as Co-Vibrations
Source: arXiv:2412.02447 source file (2025-03-10)
Supplement: Supplementary file 16 [file s5f3_moretraj_sc.tex]

%%%%%%%%%%%%%%%%%%%%%%%
%% Author: Conghao Wong
%% Date: 2024-11-04 15:06:24
%% LastEditors: Conghao Wong
%% LastEditTime: 2024-11-19 14:52:32
%% Github: https://cocoon2wong.github.io
%% Copyright 2024 Conghao Wong, All Rights Reserved.
%%%%%%%%%%%%%%%%%%%%%%%

\documentclass[../../paper.tex]{subfiles}

\begin{document}

\begin{figure}[t]
    \centering
    \includegraphics[width=1.0\linewidth]{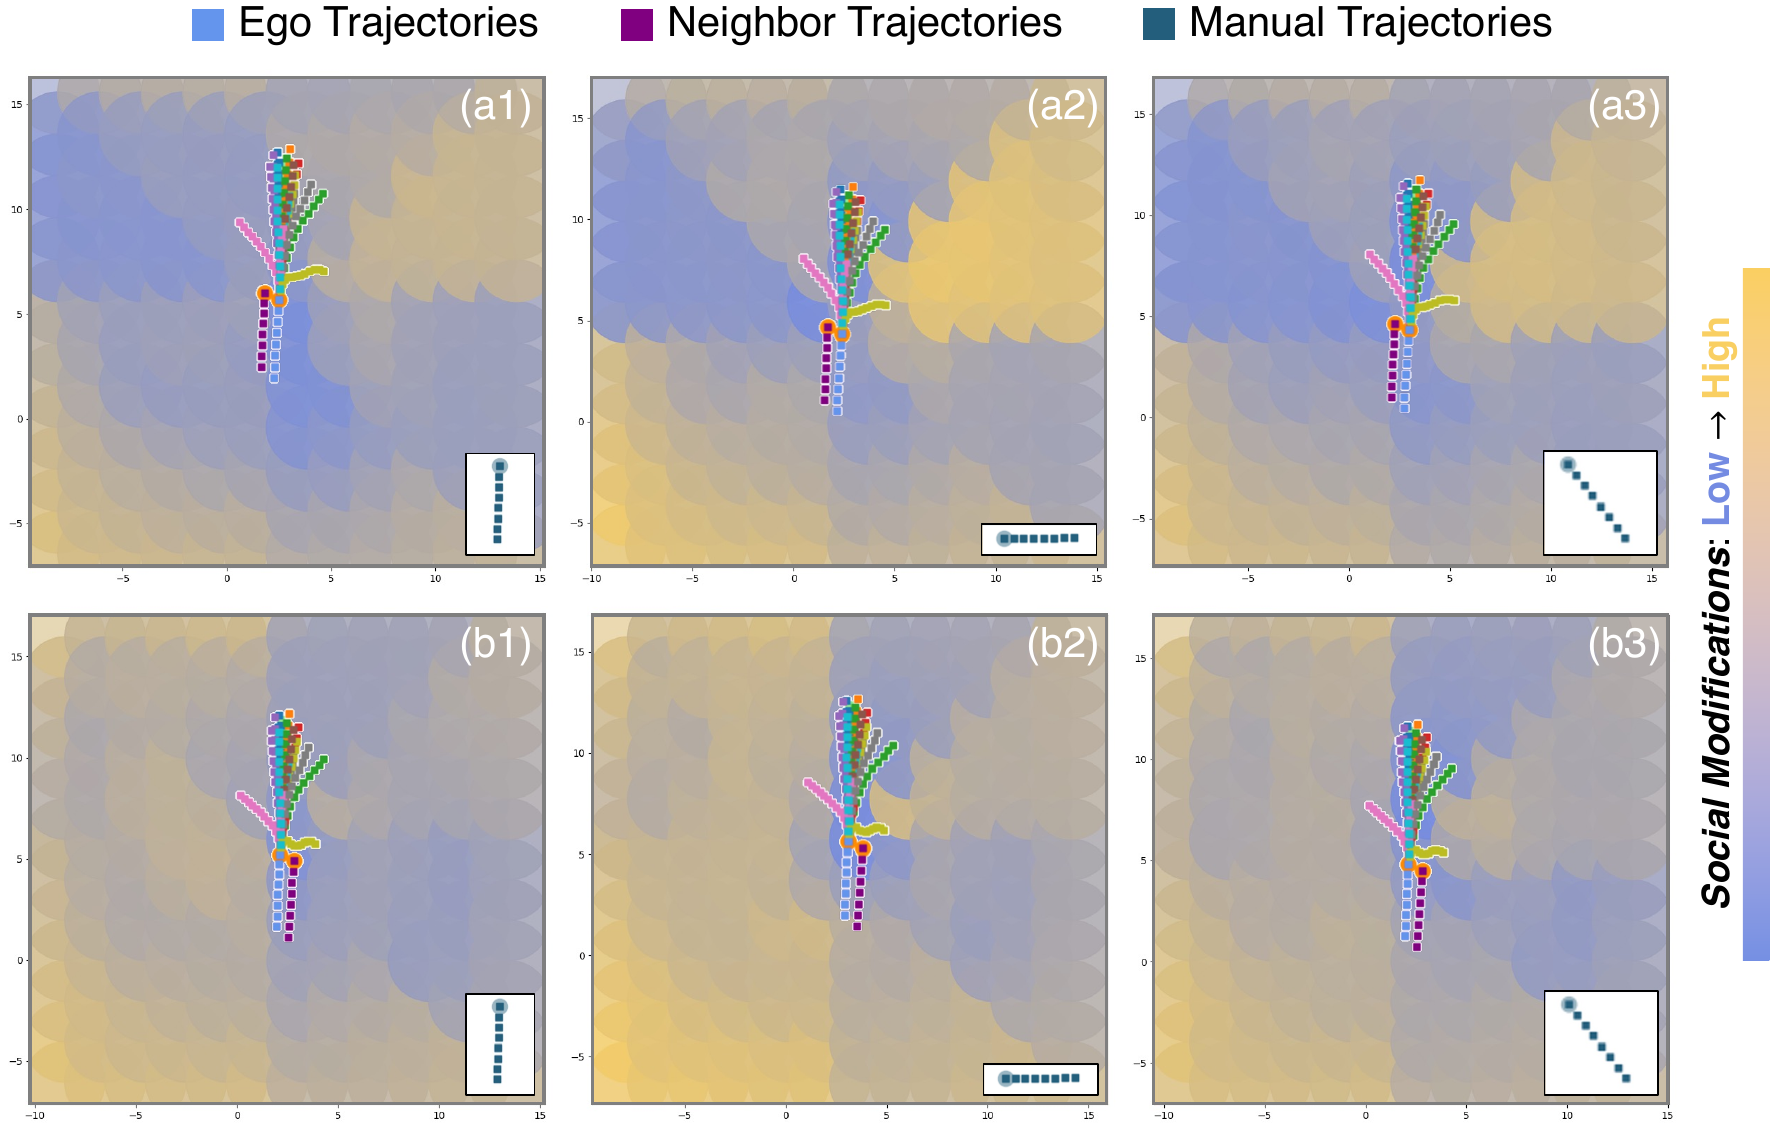}
    \caption{
        Spatial distribution $P(c(x, y | \mathbf{X}^m))$ of more structured of manual neighbors of \SCMODEL\SCCITE~model.
    }
    \label{fig_moretraj_sc}
\end{figure}

\end{document}
