# Supplementary material for: Resonance: Learning to Predict Social-Aware Pedestrian Trajectories as Co-Vibrations
Source: arXiv:2412.02447 source file (2025-03-10)
Supplement: Supplementary file 19 [file s6t2_waypoints.tex]

%%%%%%%%%%%%%%%%%%%%%%%
%% Author: Conghao Wong
%% Date: 2024-10-16 09:16:58
%% LastEditors: Conghao Wong
%% LastEditTime: 2024-11-21 17:55:17
%% Github: https://cocoon2wong.github.io
%% Copyright 2024 Conghao Wong, All Rights Reserved.
%%%%%%%%%%%%%%%%%%%%%%%

\documentclass[../../paper.tex]{subfiles}

\begin{document}

\begin{table*}[tbph]
    \centering
    \footnotesize
    \begin{tabular}{lccccccc}
        \toprule
        ID & $N_{way}$ & eth & hotel & univ & zara1 & zara2 \\

        \midrule
        c1 & 2 & 0.249/0.384 & 0.104/0.153 & 0.276/0.475 & 0.181/0.301 & 0.137/0.234 \\
        c2 & 3 & 0.236/0.362 & \C{0.102/0.150} & 0.253/0.446 & \C{0.178/0.299} & \C{0.131/0.223} \\
        c3 & 4 (default) & \C{0.232/0.354} & \C{0.103/0.152} & \C{0.242/0.414} & \C{0.172/0.290} & \C{0.131/0.225} \\
        c4 & 6 & \C{0.229/0.356} & \C{0.102}/0.154 & 0.250/0.441 & 0.182/0.310 & 0.135/0.229 \\
        c5 & 12 & 0.237/0.378 & 0.104/0.155 & \C{0.245/0.437} & 0.180/0.307 & 0.134/0.232 \\

        \bottomrule
    \end{tabular}
    \caption{
        Ablation studies on the number of waypoints $N_{way}$ when forecasting self-biases.
    }
    \label{tab_waypoints}
  \end{table*}

\end{document}
