# Supplementary material for: Resonance: Learning to Predict Social-Aware Pedestrian Trajectories as Co-Vibrations
Source: arXiv:2412.02447 source file (2025-03-10)
Supplement: Supplementary file 23 [file s7f1_biases_nuscenes.tex]

%%%%%%%%%%%%%%%%%%%%%%%
%% Author: Conghao Wong
%% Date: 2024-11-04 15:06:24
%% LastEditors: Conghao Wong
%% LastEditTime: 2024-11-21 20:42:23
%% Github: https://cocoon2wong.github.io
%% Copyright 2024 Conghao Wong, All Rights Reserved.
%%%%%%%%%%%%%%%%%%%%%%%

\documentclass[../../paper.tex]{subfiles}

\begin{document}

\begin{figure*}[t]
    \centering
    \includegraphics[width=1.0\linewidth]{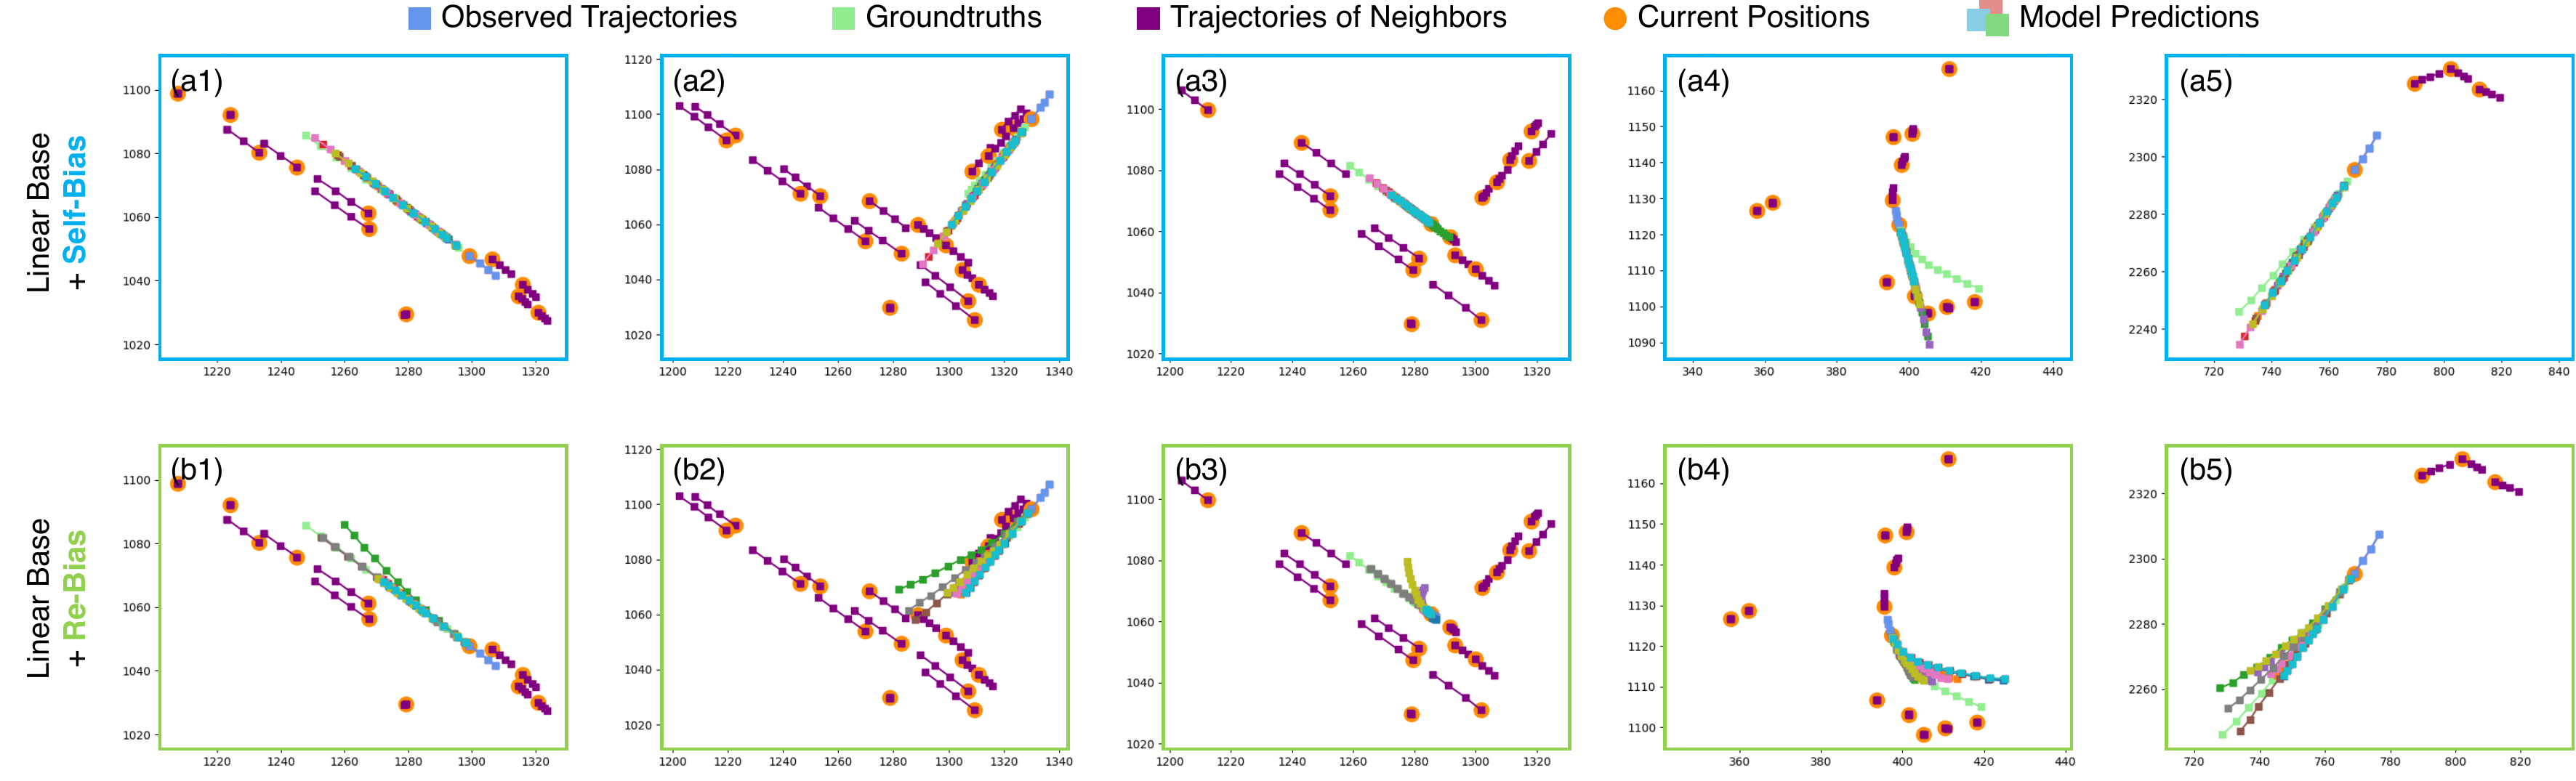}
    \caption{
        Visualized trajectory biases ($K=10$) on nuScenes.
    }
    \label{fig_biases_nuscenes}
\end{figure*}

\end{document}
