# Supplementary material for: Resonance: Learning to Predict Social-Aware Pedestrian Trajectories as Co-Vibrations
Source: arXiv:2412.02447 source file (2025-03-10)
Supplement: Supplementary file 25 [file s7t2_ab_nuscenes.tex]

%%%%%%%%%%%%%%%%%%%%%%%
%% Author: Beihao Xia
%% Date: 2025-03-08 14:22:17
%% LastEditors: Beihao Xia
%% LastEditTime: 2025-03-08 14:36:12
%% Description: file content
%% Github: https://cocoon2wong.github.io
%% Copyright 2025 Beihao Xia, All Rights Reserved.
%%%%%%%%%%%%%%%%%%%%%%%

\documentclass[../../paper.tex]{subfiles}

\begin{document}

\begin{table*}[tbph]
    \centering
    \footnotesize
    \begin{tabular}{ccc}
        \toprule
        ID & ~$l$~~$\Delta_s$~$\Delta_r$ &
        nuScenes $\downarrow$ \\

        \midrule
        a1 & \cm~~\xm~\xm       &  3.48/7.93         \\
        a2 & \cm~~\cm~\xm       &  1.26/2.36         \\
        a3 & \xm~~\xm~~SC       &  1.09/2.30         \\
        a4 & \xm~~\xm~~Re       &  \C{1.04/2.16}     \\
        a5 & \xm~~\cm~~SC       &  1.06/2.24         \\
        \bottomrule
    \end{tabular}
    \begin{tabular}{ccc}
        \toprule
        ID & ~$l$~~$\Delta_s$~$\Delta_r$ &
        nuScenes $\downarrow$ \\

        \midrule
        a6 & \xm~~\cm~~Re       &  \C{1.03/2.12}     \\
        a7 & \cm~~\xm~~SC       &  1.13/2.45         \\
        a8 & \cm~~\xm~~Re       &  1.13/2.44         \\
        a9 & \cm~~\cm~~SC       &  1.06/2.23         \\

        a0 (default) & \cm~~\cm~~Re & \X{1.05/2.17} \\
        \bottomrule
    \end{tabular}

    \caption{
        Ablation studies on nuScenes under \emph{best-of-10}.
        ``$l$'', ``$\Delta_s$'', ``$\Delta_r$'' represent whether $\hat{\mathbf{Y}}^i_l$, $\Delta \hat{\mathbf{Y}}^i_s$, and $\Delta \hat{\mathbf{Y}}^i_r$ are superposed when training.
        ``Re'' and ``SC'' denote resonance gathering and \SCMODEL~\SCPCITE~when learning $\mathbf{V}^i_r$.
        Results marked in \X{Red} denote worse ones than the best variation.
    }
    \label{tab_app_ab_nuscenes}
  \end{table*}

\end{document}
